# Supplementary material for: Social contagion and asset prices: Reddit's self-organised bull runs
Source: arXiv:2104.01847 source file (2023-08-08)
Supplement: Supplementary file 1 [file Chaotic_prices.tex]

\subsubsection{Results -- Chaotic Prices from Coordinated Strategies} 
    \label{app:chaotic_prices}
    
    We evaluate consider the implications of `coordination' and `consensus' among hype investors in two different ways. First, we theoretically determine the sensitivity of price to its various components in Eq. \ref{eq:full_price_dynamic_explained}. We subsequently perform a discrete time simulation, using parameters from the WSB forum found in section \ref{sec:social_dynamics}, to determine the price dynamics one could expect, given the current state of discussions among investors on social media. 
        
    \paragraph{Impact of $\Dot{\chi}$, $\varepsilon_{\chi}$ on Price Stability} Our original derivations offer some insight into the primary components that impact price, as explained after Eq. \ref{eq:full_price_dynamic_explained}. The influence of certain variables appears trivial to evaluate: for example, as $N$ or $M$ in Eq. \ref{eq:full_price_dynamic_explained} increase, social contagion will have greater market impact, consistently with \cite{de1990noise} who find that the fewer `sophisticated investors' there are relative to the `noise traders', the larger is the impact of noise. However, the relevance of $\Dot{\chi}$, detailed in Eq. \ref{eq:dot_phi}, and $\varepsilon_{\chi}$, detailed in Eq. \ref{eq:var_epsilon} (Appendix \ref{app:model}), is less obvious. 
          
    We turn to \cite{hommes2013behavioral} for an understanding of price stability, or instability. We consider a scenario when hype investors begin to discuss a stock but no price impact has been felt (setting $\Dot{p}/p=0$) and analyse the price dynamics that ensue. This system produces a stable steady state at $\phi = 0$ if $\hat{\alpha}/(2\hat{\theta}) \leq 1$, implying that investors are not connected enough for sentiments to amplify. In this scenario, a small value for $\hat{\alpha}/(2\hat{\theta})$ implies that consensus is difficult to reach. However, with $\hat{\alpha}/(2\hat{\theta}) >1$, we arrive at a `pitchfork' bifurcation, as described in \cite{hommes2013behavioral}. The buying intensity produces two stable steady states, $\chi^+ > 0$, $\chi^- < 0$, and one unstable steady state at $\chi^0 = 0$. These interesting dynamics illustrate the potentially important effect of strong feedback, as investors coordinate to buy or sell the asset together.
