# Supplementary material for: Social contagion and asset prices: Reddit's self-organised bull runs
Source: arXiv:2104.01847 source file (2023-08-08)
Supplement: Supplementary file 2 [file Model.tex]

\subsection{Validity of model assumptions and aggregating sentiments}
\label{app:model}

    \paragraph{Aggregating sentiments}
    %In this section, we describe how investors reach a buy/sell decision about an asset on aggregate. First, we consider that they form a sentiment $\phi_i$ about an asset based on the signals we consider in Section \ref{sec:social_dynamics}. Their choice to buy / sell the asset is modelled as a quantal response function. The precise steps are outlined here.  
    
    In Section \ref{sec:social_dynamics}, we model the log-odds of investor sentiment $\phi_i$ by a standard multivariate logistic function. This stems from a utility ranking between adopting a positive ($\phi_i = +1$) or negative ($\phi_i = -1$) position on the asset, as a function of observed returns and peer sentiment:
    \begin{align*}
        U(\phi_{i,t+1} = +1) = \epsilon_i^+ + \alpha{\phi}_{t} +\beta r_t - \gamma r_t^2, \quad 
        U(\phi_{i,t+1} = -1) =  \epsilon_i^- - \alpha{\phi}_{t} - \beta r_t - \gamma r_t^2.
    \end{align*}
    An assumption on the distribution of the idiosyncratic terms $\epsilon_i^+$ and $\epsilon_i^-$, which we state in Assumption \ref{assumption:extreme_value}, allows us to derive an expression for the probability of bullish versus bearish sentiment. We write the probability of bullish sentiment as
    \begin{align}
        \text{P}[U(+1) > U(-1)] &= \text{P}(\epsilon_i^+ + \alpha{\phi}_{t} +\beta r_t - \gamma r_t^2 > \epsilon_i^- - \alpha{\phi}_{t} - \beta r_t - \gamma r_t^2), \\
        &= \text{P}(\epsilon_i^- < \epsilon_i^+ + 2 \alpha{\phi}_{t} + 2 \beta r_t), \\ 
        &= \int_{-\infty}^{+\infty} \text{P}(\epsilon_i^- < \epsilon_i^+ + 2 \alpha{\phi}_{t} + 2 \beta r_t | \epsilon_i^+) \times p(\epsilon_i^+) d\epsilon_i^+, \\
        &= \int_{-\infty}^{+\infty} \text{exp}\left[ -\text{exp}\left(- \frac{\epsilon_i^+ + 2\alpha{\phi}_{t} + 2\beta r_t}{2\lambda} \right) \right] \times \frac{1}{2\lambda}\text{exp}\left[ - \frac{\epsilon_i^+}{2\lambda} -\text{exp}\left(- \frac{\epsilon_i^+}{2\lambda} \right)  \right] d\epsilon_i^+, \label{eq:probability_density_assumption} \\
        &= \frac{\text{exp}\left(\frac{\alpha{\phi}_{t} + \beta r_t}{\lambda}\right)}{\text{exp}\left( \frac{\alpha{\phi}_{t} + \beta r_t}{\lambda}\right) + 1},
    \end{align}
    where step \ref{eq:probability_density_assumption} follows from the fact that we are integrating the cumulative density of $\epsilon_i^-$, with scale $2\lambda$, over the support of $\epsilon_i^+$, with marginal density with marginal density $p(\epsilon) = \text{exp}[-\epsilon/2\lambda -\text{exp}(-\epsilon/2\lambda)]/2\lambda$. The final simplification comes from the fact that $U(\phi_{i,t+1} = +1)$ and $U(\phi_{i,t+1} = -1)$ are symmetric in parameters $\alpha, \beta$ and $\gamma$. If we want to keep them distinct, we arrive at the quantal response function for the probability of positive or negative sentiment:
    \begin{align*}
          \phi_{i,t+1}^D =
          \begin{cases}
          +1, & \text{with probability} \frac{\text{exp}\left[(\alpha{\phi}_{t} +\beta r_t - \gamma r_t^2)/2\lambda\right]}{\text{exp}\left[( \alpha{\phi}_{t} + \beta r_t - \gamma r_t^2)/2\lambda\right] + \text{exp}\left[( -\alpha{\phi}_{t} - \beta r_t - \gamma r_t^2)/2\lambda\right]}, \\
          -1, & \text{with probability } \frac{\text{exp}\left[( -\alpha{\phi}_{t} - \beta r_t - \gamma r_t^2)/2\lambda\right]}{\text{exp}\left[( \alpha{\phi}_{t} + \beta r_t - \gamma r_t^2)/2\lambda\right] + \text{exp}\left[(-\alpha{\phi}_{t} - \beta r_t - \gamma r_t^2)/2\lambda\right]}.
          \end{cases}
    \end{align*}
    Therefore, we can model the aggregate buying intensity by summing $\phi_{i,t+1}^D$ across the $N$ hype investors, which yields the well-known hyperbolic tangent function: 
    \begin{align*}
        \phi_{t+1} = \text{tanh}\left[ (\beta r_t + \alpha \phi_{t})/\lambda \right].
    \end{align*}
    Our Online Appendix includes additional details on the properties of this function.
    % \begin{figure}[ht]
    %     \begin{center}
    %      \includegraphics[width=0.5\linewidth]{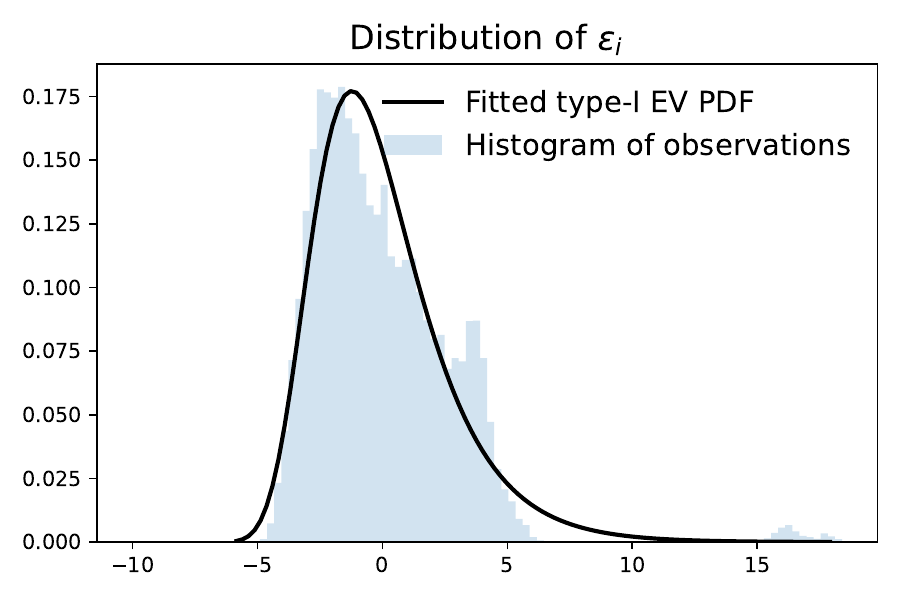}
    %      \caption{\textbf{Distribution of $\epsilon_i$}; We plot the observed distribution of residuals from the regressions presented in Eq. \ref{eq:epsilon_i}, which we use to estimate author's $\epsilon_i$. We overlay our histogram of observations with a fitted type-I error distribution Probability Density Function (PDF). The location parameter for our fitted type-I EV is $-1.22$ and the scale parameter is $2.08$}
    %      \label{fig:dist_epsilons}
    %     \end{center}
    % \end{figure}    

    \paragraph{Validity of Assumption \ref{assumption:other_investors}}  \citet{shiller1984stock} demonstrates that fully `rational investors' (a category of investor we liken to non-hype investors in this paper) would anticipate persistent shifts in hype investors' demand for a stock, potentially justifying their willingness to pay a price different from that derived by discounting a stream of dividends. Our assumption is, therefore, somewhat reasonable as it implies that non-social investors hold the asset at every price point, and simply trade to keep their exposure constant. 
    
    \paragraph{Validity and implications of Assumption \ref{assumption:capacity}} We consider a shift in the number of hype investors $N$ to be exogenous for the purposes of this section. We also hold the ratio $M/p_t$ constant: this implies that the balances hype investor have invested in the asset, $M$, increase and decrease proportionally with the asset's price. Any changes in price are met with proportional profits / decreases in capital $M$ -- potentially due to gains from investments or moving capital elsewhere, allowing us to keep the ratio $M/p_t$ fixed.
