# Supplementary material for: Social contagion and asset prices: Reddit's self-organised bull runs
Source: arXiv:2104.01847 source file (2023-08-08)
Supplement: Supplementary file 3 [file Model_stability_analysis.tex]

%In this section of the appendix, we discuss the methodology behind Section \ref{subsec:stability_analysis}. We precisely outline the steps taken to find our system steady states, as well as show the expected system behaviour around the steady states. 
\subsection{Stability Analysis}
\label{app:stability_analysis}

As mentioned in Section \ref{subsec:stability_analysis}, $r_t$ must be zero at the steady state. This means that steady states of the dynamic system in Eqs. \ref{eq:consensus_model_discrete_1}-\ref{eq:consensus_model_discrete_2} are those for which $\phi_t$ is a solution to Eq. \ref{eq:consensus_model_discrete_1}. Due to the properties of the hyperbolic tangent function (explored thoroughly in the Online Appendix), zero is a unique steady state when $\alpha/\lambda <1$, and two further steady states emerge when $\alpha/\lambda > 1$. Those two additional steady states are solved numerically in all simulation exercises, using a solving algorithm.

The behaviour of our system depends not only on the existence of steady states, but also on the types of steady states that we observe in different stability regions. In a discrete time system, the type of stability around a steady state is dependent on the eigenvalues of the Jacobian matrix at the steady state. The Jacobian matrices at the different steady states are %Table \ref{tab:jacobian_steady_states} shows some types of common behaviours around a single steady state, as they relate to the Jacobian eigenvalues. When a system has multiple eigenvalues, different behaviours can emerge. For example, if we consider two eigenvalues $x_1$ and $x_2$ and $|x_1| > 1$ while $x_2 <1$, we would observe a saddle. Various resources exist to review system steady states, largely originating from the study of physical systems, with \cite{hommes2013behavioral} providing a relevant review for the economic setting.

\begin{align}
    J(0,0) =    \begin{bmatrix} 
            	\alpha & \beta \\
            	C(\alpha - 1) & C\beta
            	\end{bmatrix}, \quad
    J(\phi,0) = \begin{bmatrix} 
            	\alpha \text{sech}^2(\alpha\phi) & \beta \text{sech}^2(\alpha\phi) \\
            	C\left(\alpha\text{sech}^2(\alpha\phi) - 1\right) & C\beta \text{sech}^2(\alpha\phi)
            	\end{bmatrix},
\end{align}
where $\phi \in \{\phi^+, \phi^-\}$. The corresponding eigenvalues for steady state $(0,0)$ are
\begin{align}
\label{eq:eigenvalue_0_0}
    x_1 = \frac{1}{2} \left( C\beta + \alpha + \sqrt{(C\beta + \alpha)^2 - 4C\beta} \right), \quad
    x_2 = \frac{1}{2} \left( C\beta + \alpha - \sqrt{(C\beta + \alpha)^2 - 4C\beta} \right),
\end{align}
and those for steady states $(\phi,0)$ are
\begin{align}
\label{eq:eigenvalue_phi_0_plus}
    x_1 = \frac{\text{sech}^2(\alpha\phi)}{2} \left((C\beta + \alpha) + \sqrt{\text{sech}^2(\alpha\phi)(C\beta + \alpha)^2 - 4C\beta} \right), \\
    x_2 = \frac{\text{sech}^2(\alpha\phi)}{2} \left((C\beta + \alpha) - \sqrt{\text{sech}^2(\alpha\phi)(C\beta + \alpha)^2 - 4C\beta} \right). \label{eq:eigenvalue_phi_0_minus}
\end{align}
These expressions trace different regions of stability as a function of $C\beta$ and $\alpha$ in Figure \ref{fig:stability_regions}. 

Figure \ref{fig:stability_regions} is drawn by solving numerically for the points $C\beta$ for which the eigenvalues in Eq. \ref{eq:eigenvalue_0_0}, on the left, and Eqs. \ref{eq:eigenvalue_phi_0_plus}-\ref{eq:eigenvalue_phi_0_minus}, on the right, switch between the different stability regions. Specifically, we solve for when the complex part of the eigenvalues is equal to zero, and the eigenvalues are on the unit circle. These points are computed by taking a range of values for $\alpha$, then applying a solving algorithm. The solutions are used to distinguish the different regions of stability in Figure \ref{fig:stability_regions}.
