# Supplementary material for: Social contagion and asset prices: Reddit's self-organised bull runs
Source: arXiv:2104.01847 source file (2023-08-08)
Supplement: Supplementary file 4 [file Simulation.tex]

% \newpage

\subsection{Asset Price Simulation}
\label{app:simulation}

    \paragraph{Discrete Time Simulation} We perform a discrete time simulation of our final model, presented in Eq. \ref{eq:full_price_dynamic_explained}.
        
    The choices made to simulate the model include: i) some fixed fraction of hype investors, $a_0$, are always present with a fixed buying intensity, and ii) non-hype investors fix the nominal value of their investment. In practice this implies that hype investors enter the market to buy the asset (since $\phi_0>0$), which other investors sell to them at a higher price. The price changes and coordination of buying strategies affect the intensity with which hype investors purchase the asset in subsequent periods. Gradually, they leave the market until only the starting amount $a_0$ remain, and the price returns to its `true' value.
        
        \begin{figure}[ht!]
            \begin{subfigure}{0.5\textwidth}
                \centering
                \includegraphics[width=\linewidth]{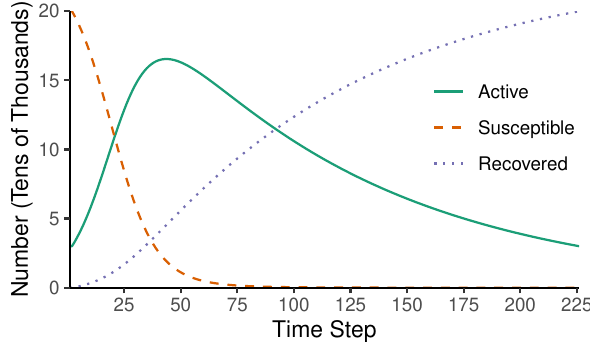}
                \caption{Contagion among Hype Investors} 
                \label{fig:contagion_plot}
            \end{subfigure}
            \hfill
            \begin{subfigure}{0.5\textwidth}
                \centering
                \includegraphics[width=\linewidth]{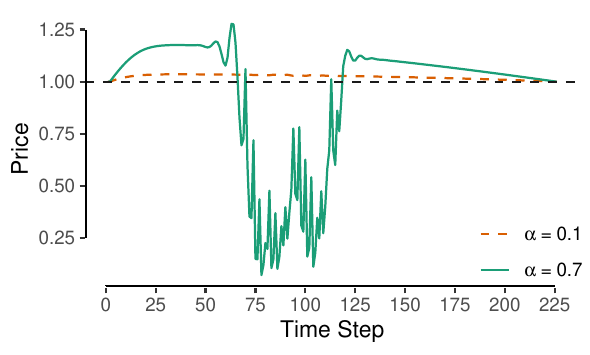}
                \caption{Impact on Price} 
                \label{fig:price_plot_baseline}
            \end{subfigure}
            \bigskip
            \begin{subfigure}{0.5\textwidth}
                \centering
                \includegraphics[width=\linewidth]{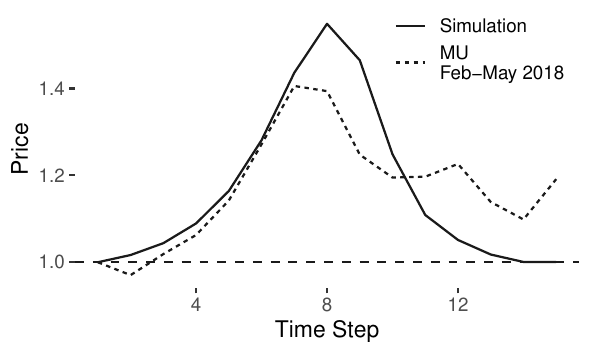}
                \caption{MU Observed and Simulated Price Dynamics} 
                \label{fig:contagion_MU}
            \end{subfigure}
            \hfill
            \begin{subfigure}{0.5\textwidth}
                \centering
                \includegraphics[width=\linewidth]{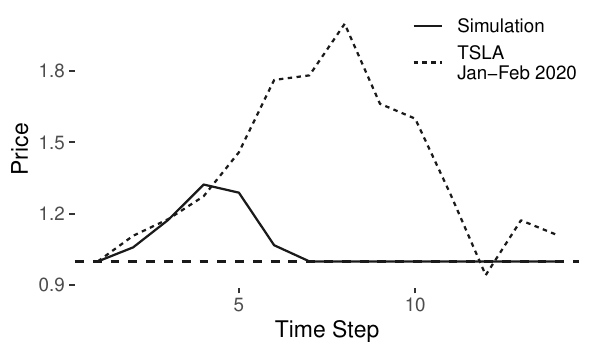}
                \caption{TSLA Observed and Simulated Price Dynamics} 
                \label{fig:contagion_TSLA}
            \end{subfigure}
            \caption{\textbf{Price Impact of Contagion and Opinion Dynamics}; In Figures \ref{fig:contagion_plot}, \ref{fig:price_plot_baseline} we illustrate the hypothetical dynamics that can emerge within our model. On the left, the number of active hype investors in an asset increases steeply until time step 50, after which the number slowly declines to its initial value (as `active' investors `recover'). On the right, at price first increases until time step 50, after which it experiences a volatile crash when consensus formation is strong ($\alpha = 0.7$), then returns to its initial level. In contrast, when consensus formation is weak ($\alpha = 0.1$), very little price impact is observed. Other parameter choices are discussed in Appendix \ref{app:simulation}. Figure \ref{fig:contagion_MU}, \ref{fig:contagion_TSLA} show the dynamics simulated using parameters derived from WSB in the two stocks at a time when the tickers were increasing in popularity within the forum. The stock price displayed is the average weekly close price for each stock (ensuring consistent time steps between asset price and simulation).}
            \label{fig:price_baseline}
        \end{figure}
        
        Since the focus is on asset demand by hype investors, we simulate various parameters for coordination, $\alpha$. Given the complex dynamics, qualitatively different patterns could be generated depending on the choice of demand parameters. The result, in Figure \ref{fig:price_plot_baseline}, displays three important characteristics for scenarios where consensus is strong ($\alpha = 0.7)$ and weak ($\alpha = 0.1)$; other parameters are chosen in line with empirical observations and discussed further below. Under strong consensus, the initial increase in demand, until time step 50, gradually drives up price. Once this growth is depleted, the price crashes dramatically, and extreme volatility persists until time step 150. At this stage, some active investors still remain in the market, but the price follows a steady downward trend until it reaches its initial level. In contrast, the effect under weak consensus is relatively mute, as new entrants fail to adopt the sentiments of existing investors.
        These findings support the conclusions in \cite{de1990noise}, stating that if `sophisticated investors' time horizons are long, compared to `noise traders', they can `buy low, confident that they will be able to sell high when prices revert to the mean'. Eventually, the asset's price reverses to its original level as hype investors exit the market and other investors trade to revert the asset to its fundamental value. 
        
        Figures \ref{fig:contagion_MU}, \ref{fig:contagion_TSLA} on the other hand consider the dynamics that our model implies for two popular stocks within the WSB forum. We initiate the model with coordination and contagion parameters from our data. We emphasize that our goal is not to show that our model can predict stock price movements, but rather that stock price fluctuations, indeed, appear to follow a bursty pattern, consistent with our model and contagion / consensus among hype investors. We observe that in our TSLA simulation, we significantly under-predict the price change. This may be due to our under-estimation of of the number of hype-investors versus other investors, or the fact that following a significant price increase, other investors also change their dynamics. 
