# Supplementary material for: Social contagion and asset prices: Reddit's self-organised bull runs
Source: arXiv:2104.01847 source file (2023-08-08)
Supplement: Supplementary file 5 [file Topic_model.tex]

\subsection{Topic model}
\label{app:topic_model}

         \begin{figure}[ht]
             \begin{center} 
                 \includegraphics[width=\textwidth]{Figures/topic_model.pdf} 
                 \caption{\textbf{Temporal trends in topics}; the stacked count, normalized to 100\% at each time period, showing the prevalence of a select subset of topics discussed on WallStreetBets.}
                 \label{fig:topic_hist}
             \end{center}
         \end{figure} 

        Does WSB reflect new information for the larger market to trade on, or social activity that drives perceived changes in value, regardless of fundamentals? A topic model offers a simple method to evaluate the content of WSB discussions. Figure \ref{fig:topic_hist} presents our preferred topic model, namely the Biterm Topic Model (BTM), which is optimal for smaller bodies of text \citep{yan2013biterm}. Submissions from April 2012 to February 2021 give a time series of almost 100 months. A random sample of submissions is drawn for the months of January and February 2021 in order to prevent these two months, with a high number of submissions, from skewing the topic model results. 
        
        Figure \ref{fig:topic_hist} presents a stacked plot of the monthly submission count of a selected subset of discussions, normalised by the total across the selected topics. It begins in 2015 when the forum gained a consistent user base. On one hand, some topics persist in the overall discussion: people consistently ask for advice about trading accounts and anonymously share details of how their trading is affecting their personal lives. On the other hand, topics concerned with larger economic trends wax and wane over the observation period. Two examples of this are the uptick in submissions discussing GME and Roinhood account trading limits, coinciding with the GME short squeeze, and the COVID-19 topic, which is negligible until January 2020, but gains prominence in the subsequent months. Pharmaceutical company and natural resource discussions, on the other hand, seem to loose popularity. A full list of topics with their respective keywords is presented below.
        
\clearpage

    \begin{table}[!htbp]
    {
    \centering
    \begin{tabular}{|c|c|c|}
    \hline
    \textbf{Topic Title} & \textbf{Top Words} & \textbf{Topic Prevalence (\%)} \\
    \hline
Robinhood Trading Limits & \multicolumn{1}{m{8cm}|}{robinhood, gme, account, nkla, margin, order, app, limit, broker, orders} & 1.8 \\
 \hline 
International Trade & \multicolumn{1}{m{8cm}|}{expected, yr, china, usd, europe, japan, pmi, manufacturing, korea, data} & 0.8 \\
 \hline 
Retail Sales + Amazon & \multicolumn{1}{m{8cm}|}{sales, amazon, home, stores, business, online, companies, food, store, retail} & 3.0 \\
 \hline 
Top Stock Picks / Positions & \multicolumn{1}{m{8cm}|}{tsla, news, sold, aapl, weeks, holding, hold, amd, months, dip} & 11.6 \\
 \hline 
Other & \multicolumn{1}{m{8cm}|}{comments, daily, best, moves, spy, weekend, fo, fn, fm, fp} & 1.1 \\
 \hline 
Other & \multicolumn{1}{m{8cm}|}{mentions, vote, log, wsbvotebot, submission, posts, check, reverse, mention, great} & 0.2 \\
 \hline 
Electric Cars & \multicolumn{1}{m{8cm}|}{tsla, energy, car, ev, cars, nio, electric, battery, elon, space} & 2.3 \\
 \hline 
Revenues, Earnings, Ratings & \multicolumn{1}{m{8cm}|}{revs, beats, tgt, line, eps, neutral, downgraded, initiated, fy, reports} & 0.9 \\
 \hline 
FDA / Pharma & \multicolumn{1}{m{8cm}|}{drug, fda, phase, patients, vaccine, trial, treatment, results, clinical, covid} & 2.9 \\
 \hline 
Revenues, Earnings, Ratings & \multicolumn{1}{m{8cm}|}{revenue, million, growth, quarter, share, sales, billion, net, expected, eps} & 4.0 \\
 \hline 
China Trade Deal & \multicolumn{1}{m{8cm}|}{trump, china, said, president, deal, bill, house, election, chinese, news} & 3.1 \\
 \hline 
Social Media Stocks & \multicolumn{1}{m{8cm}|}{fb, game, snap, aapl, disney, games, video, google, users, netflix} & 2.7 \\
 \hline 
GME Discussion & \multicolumn{1}{m{8cm}|}{companies, gme, investors, world, years, believe, hedge, actually, value, funds} & 7.3 \\
 \hline 
Financial News & \multicolumn{1}{m{8cm}|}{data, information, news, financial, report, based, find, sec, research, investors} & 4.3 \\
 \hline 
Personal Discussions & \multicolumn{1}{m{8cm}|}{life, wife, ass, little, said, spy, getting, old, red, went} & 7.6 \\
 \hline 
Weed Stocks & \multicolumn{1}{m{8cm}|}{million, share, capital, ceo, cannabis, ipo, public, management, merger, billion} & 2.1 \\
 \hline 
     \end{tabular}
    \caption{\textbf{Topics Extracted from BTM Model (1)}}
    \label{table::btm_topics1}}
    \end{table}
    \begin{table}[!htbp]
    \begin{center}
    \begin{tabular}{|c|c|c|}
    \hline
    \textbf{Topic Title} & \textbf{Top Words} & \textbf{Topic Prevalence (\%)} \\
    \hline
Software Tech Stocks & \multicolumn{1}{m{8cm}|}{amd, aapl, intc, companies, data, cloud, software, technology, services, tech} & 3.4 \\
 \hline 
Earnings Release & \multicolumn{1}{m{8cm}|}{release, estimates, consensus, share, revenue, move, open, beat, average, interest} & 1.0 \\
 \hline 
Natural Resources & \multicolumn{1}{m{8cm}|}{oil, gold, prices, silver, gas, futures, crude, production, demand, companies} & 1.8 \\
 \hline 
FED / Rates & \multicolumn{1}{m{8cm}|}{fed, rates, rate, economy, markets, economic, said, interest, growth, inflation} & 6.0 \\
 \hline 
Other Tech Stocks & \multicolumn{1}{m{8cm}|}{tsla, pltr, elon, musk, mods, ban, gme, retards, gains, autists} & 2.0 \\
 \hline 
COVID / China & \multicolumn{1}{m{8cm}|}{virus, covid, cases, coronavirus, china, world, weeks, corona, states, news} & 4.8 \\
 \hline 
Other & \multicolumn{1}{m{8cm}|}{spy, bear, gay, text, bears, bull, gang, msft, words, stonks} & 1.7 \\
 \hline 
Debt / Loans & \multicolumn{1}{m{8cm}|}{debt, cash, pay, credit, loans, loan, million, interest, billion, bank} & 3.4 \\
 \hline 
Other & \multicolumn{1}{m{8cm}|}{usd, bln, exp, revenue, newswires, eps, co, share, symbol, live} & 1.4 \\
 \hline 
Other & \multicolumn{1}{m{8cm}|}{spy, chart, close, index, month, performance, major, past, futures, sectors} & 1.3 \\
 \hline 
Account Help & \multicolumn{1}{m{8cm}|}{account, help, investing, best, start, robinhood, advice, work, years, please} & 7.4 \\
 \hline 
Other & \multicolumn{1}{m{8cm}|}{spy, volume, chart, support, bullish, low, trend, resistance, bearish, line} & 3.7 \\
 \hline 
Other & \multicolumn{1}{m{8cm}|}{amet, calendar, releases, wed, link, thurs, tues, fri, analyst, close} & 0.5 \\
 \hline 
Options / Risk & \multicolumn{1}{m{8cm}|}{option, spy, profit, strike, spread, risk, loss, value, selling, position} & 6.3 \\
 \hline 
     \end{tabular}
    \end{center}
    \caption{\textbf{Topics Extracted from BTM Model (2)}}
    \label{table::btm_topics2}
    \end{table}
