# Supplementary material for: Social contagion and asset prices: Reddit's self-organised bull runs
Source: arXiv:2104.01847 source file (2023-08-08)
Supplement: Supplementary file 6 [file bifurcation_diagrams_alpha.tex]

\subsection{Bifurcation diagram with respect to consensus}
\label{app:bifurcation_alpha}

    \begin{figure}[!htbp]
        \begin{subfigure}{\textwidth}
            \centering
            \includegraphics{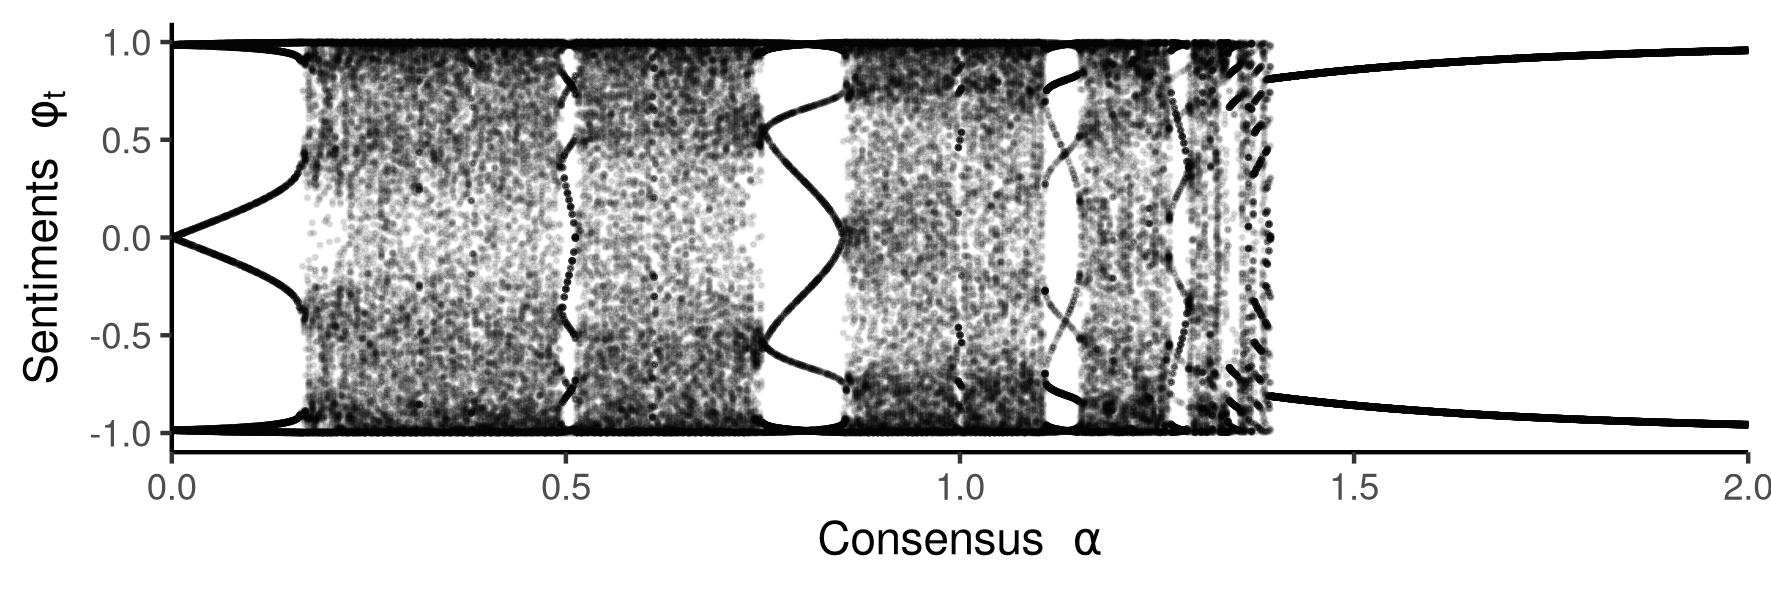}
            \caption{$C = 2.5$} 
            \label{fig:phi_bifurcation_diagram_high_beta}
        \end{subfigure}

        \begin{subfigure}{\textwidth}
            \centering
            \includegraphics{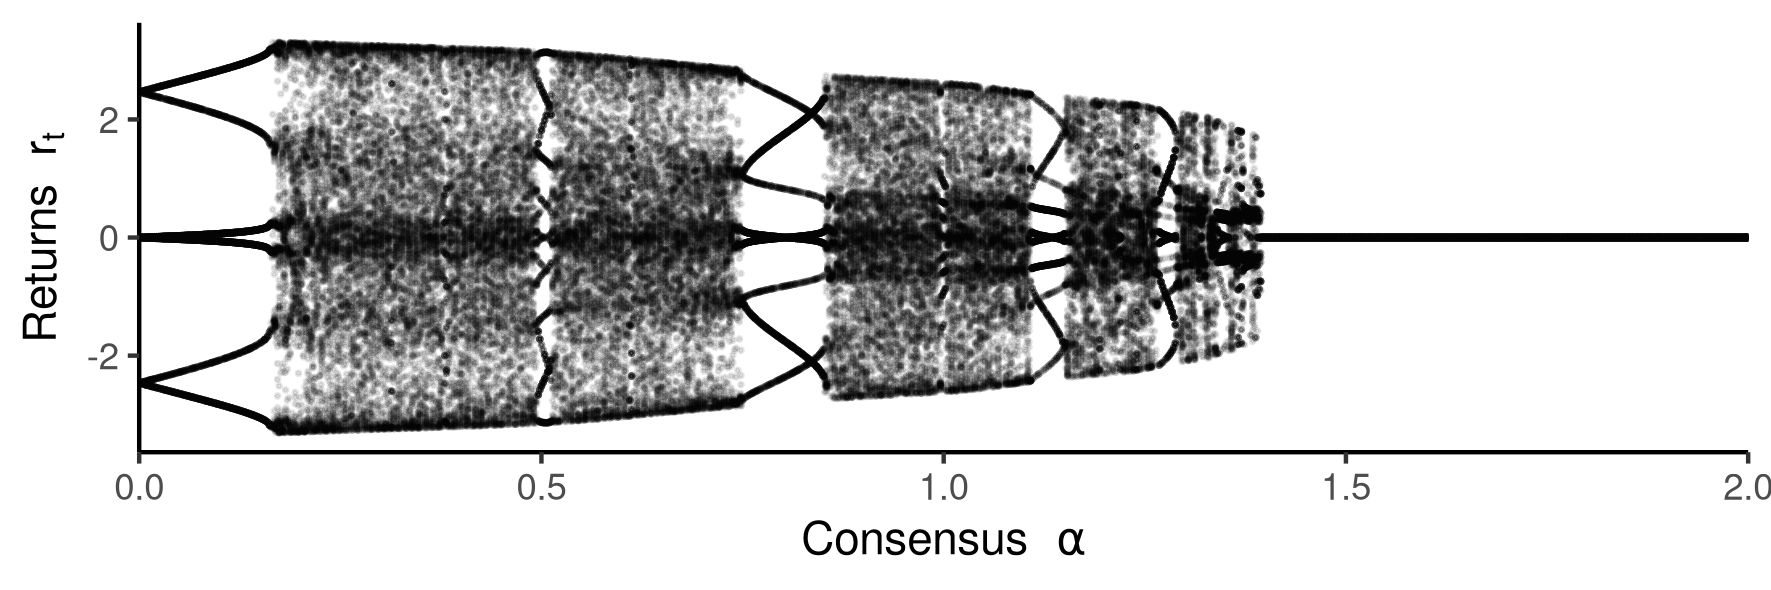}
            \caption{$C = 2.5$} 
            \label{fig:return_bifurcation_diagram_high_beta}
        \end{subfigure}
        
        \begin{subfigure}{\textwidth}
            \centering
            \includegraphics{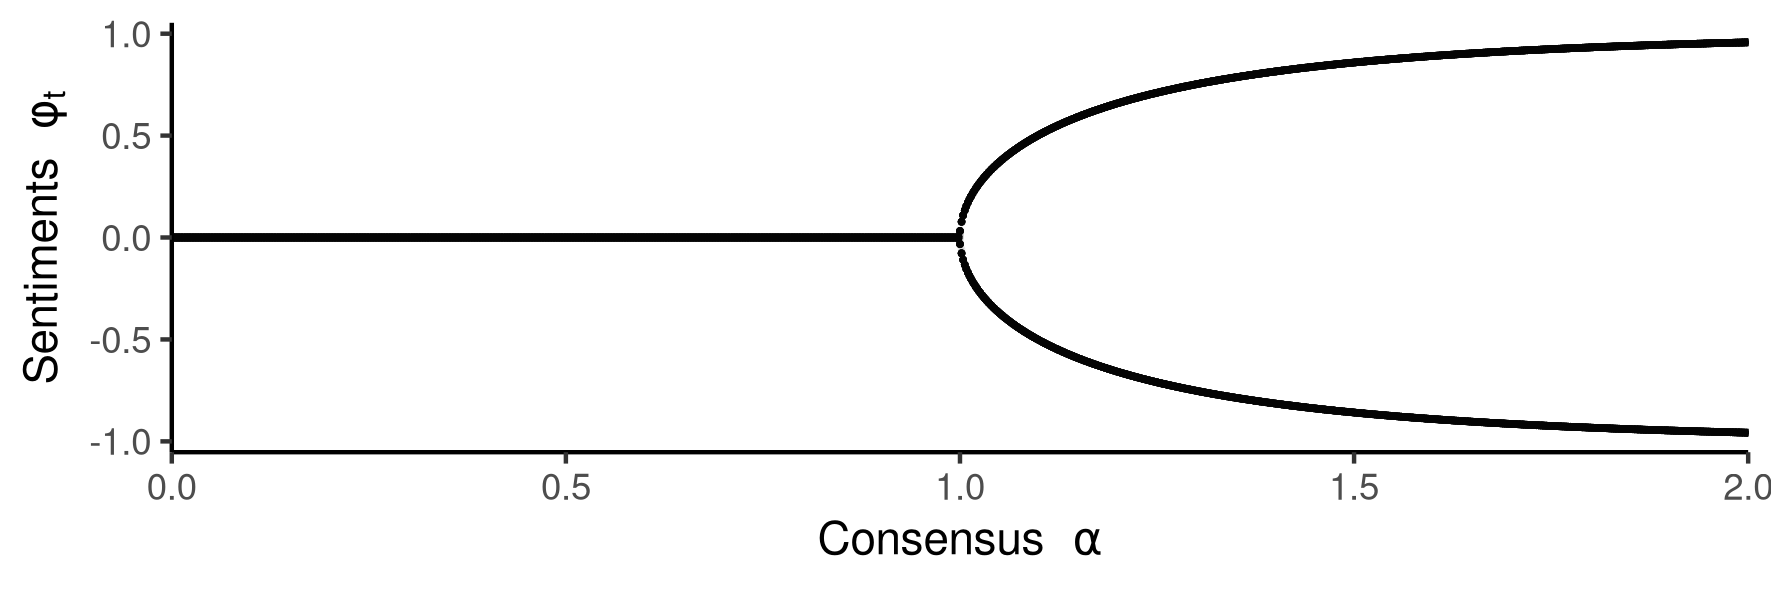}
            \caption{$C = 0.3$} 
            \label{fig:phi_bifurcation_diagram_low_beta}
        \end{subfigure}

        \begin{subfigure}{\textwidth}
            \centering
            \includegraphics{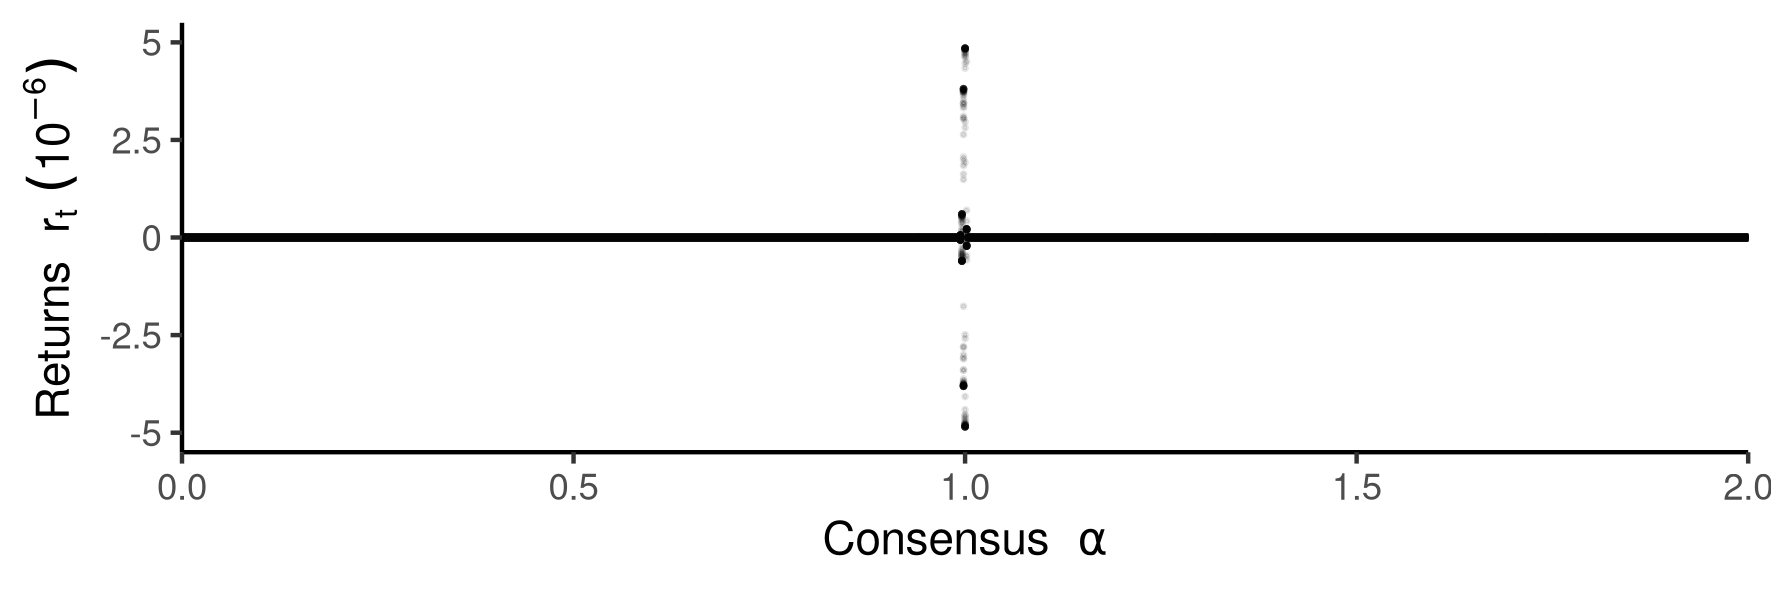}
            \caption{$C = 0.3$} 
            \label{fig:return_bifurcation_diagram_low_beta}
        \end{subfigure}
        
        \caption{\footnotesize{\textbf{Bifurcation diagrams with respect to consensus parameter $\alpha$}; the final values from one thousand iterations of the dynamic system in Eqs. \ref{eq:consensus_model_discrete_1}-\ref{eq:consensus_model_discrete_2}, are plotted, for two values of $C$ (2.5 and 0.3) and a range of values for $\alpha$ between zero and two. Remaining parameters are constant for $\beta = 1$ and $\lambda = 1$. One hundred initial values for $r$ are drawn from a normal distribution with mean zero and variance 0.25, with $\phi$ initiated at zero.}}
        \label{fig:bifurcation_diagram_alpha}
    \end{figure} 
    
    We produce two additional bifurcation diagrams for each state variable, varying $\alpha$. Figure \ref{fig:stability_regions} suggests two interesting values for $C$ -- one at 0.3, and a second at 2.5. We assign parameter $\beta$ a value of one. We then initialise sentiment $\phi_0$ to be zero, and randomly draw one hundred values for returns $r_0$ from a normal distribution with mean zero and variance 0.25. For a set of values of $\alpha$, ranging from zero to two, we iterate forward $\phi_t$ and $r_t$ one thousand times. The final values for $\phi_t$ and $r_t$ are then plotted as a function of $\alpha$.
    
    Those plots are presented in Figure \ref{fig:bifurcation_diagram_alpha}. Figure \ref{fig:phi_bifurcation_diagram_high_beta} illustrates the final values for $\phi_t$ when $C$ is set to 2.5, and Figure \ref{fig:return_bifurcation_diagram_high_beta} does the same for $r_t$. For low values of $\alpha$, sentiments, and concurrently returns, display quasi-periodic dynamics (in the clouded regions), interrupted by stable cycles (for example when $\alpha$ is around 0.8). Larger values of $\alpha$ eventually dominate the effect of hype investors' large capacity, and the system settles at it steady states, with either positive or negative sentiment. This in stark contrast to a scenario where capacity is too small, as in Figures \ref{fig:phi_bifurcation_diagram_low_beta} and \ref{fig:return_bifurcation_diagram_low_beta} where $C$ is set to 0.3. The meaningful change in the behaviour of the system is that sentiments settle at one value, either positive or negative, when $\alpha$ is greater than one -- already present in the one-dimensional hyperbolic tangent map from Figure \ref{fig:bifurcation_1_D}. It is interesting to note that there is slight residual dispersion in returns in Figure \ref{fig:return_bifurcation_diagram_low_beta} (note the scale of the axis) when $\alpha$ reaches that threshold, as one steady state loses its stability, and two new ones barely emerge.
