# Supplementary material for: Social contagion and asset prices: Reddit's self-organised bull runs
Source: arXiv:2104.01847 source file (2023-08-08)
Supplement: Supplementary file 7 [file Consensus_network.tex]

\subsection{Aggregate Opinion Formation}
\label{app:consensus_network}

        \input{Tables/leontieff_sentiment_spillovers}
        
        One pertinent question is on the persistence of aggregate opinions. This is of particular importance when considering market impact: do investors come to an agreement about whether an asset should be bought or sold? We estimate this phenomenon through a parameter $\alpha$, which denotes the aggregate buying/selling intensity resulting from individual opinion formation.
        
        One way gauge $\alpha$ is to replace matrix $\boldsymbol{W}$ in Eqs. \ref{eq:network_model1}-\ref{eq:network_model2} by its Leontief inverse, $(\boldsymbol{I}-\boldsymbol{W})^{-1}$. Instead of a weighted average of $i$'s direct neighbours, the Leontief inverse returns the overall position of user $i$ in the network. While immediate neighbours are still highly weighted, the sentiments of their neighbours, and those neighbours' neighbours, feature as well. The end result is that $(\boldsymbol{I}-\boldsymbol{W})^{-1}$ captures the sentiments related to an asset in the broader context of the whole forum, appropriately discounting those further removed from $i$.
        
        The first two columns in Table \ref{tab:leontieff_sentiment_spillovers} show the coefficients of Eq. \ref{eq:network_model2}, but with the adjacency matrix replaced by its Leontief inverse, and the diagonal elements set to zero. The baseline coefficients are suppressed, since they do not vary substantially from Table \ref{tab:adjacent_sentiment_spillovers}. The stark difference here is the much stronger effect of volatility, $(\boldsymbol{I}-\boldsymbol{W})^{-1} \sigma$. It reflects a strong persistence of bearish sentiments in discussions when the asset in question experiences volatility. In contrast to the statistically insignificant coefficient on overall returns, $(\boldsymbol{I}-\boldsymbol{W})^{-1} R^e$, volatility, and the panic it appears to induce, has a powerful, propagating effect in the formation of investor opinions in WSB.
        
        The final set of columns in Table \ref{tab:leontieff_sentiment_spillovers} investigate whether sentiments detected in users who post their first submission, versus those that have already expressed an opinion in the past, are noticeably different. The answer is affirmative; interacting the relevant dummy variable with the spillover term, $(\boldsymbol{I}-\boldsymbol{W})^{-1} \boldsymbol{\phi^s} \times \phi^{NA}_{-1}$, demonstrates that the large bearish spillovers take hold in users who post for the first time. The original coefficient, $(\boldsymbol{I}-\boldsymbol{W})^{-1} \boldsymbol{\phi^-}$, is statistically insignificant in predicting bearish over neutral sentiment, while those for bullish sentiment are largely in the same direction.
