# Supplementary material for: Social contagion and asset prices: Reddit's self-organised bull runs
Source: arXiv:2104.01847 source file (2023-08-08)
Supplement: Supplementary file 8 [file Data.tex]

\newpage

\subsection{Data Appendix}
\label{app:data_appendix}

    Besides the scraped text data from Reddit, we downloaded historical price series on extracted tickers from The Center for Research on Security Prices (CRSP). The time period, denoted by $t$, is defined as the 24 hours between closing times on the New York Stock Exchange, namely 4pm EST. For example, a submission made on Tuesday at 5pm EST is categorised in the same time frame as a submission made on the following Wednesday at 10am. This is done to mitigate any influence that news occurring outside market hours might have on WSB conversations. The choice of timing may not be consistent with non-US stock markets, but, given that almost all discussed assets are US stocks and indices, this does not impact our findings. The financial data used are: $P_{i,t}$, the dollar price of security $i$ at closing time of day $t$, $R^f_t$, the risk-free rate of return obtained from Kenneth R. French's data library, $(P^H_{i,t},P^L_{i,t})$, the intra-day high and low prices of security $i$ at closing time of day $t$, and $V_{i,t}$, the trading volume of security $i$ at closing time of day $t$.
    
    We computed the variables for Table \ref{tab:submission_time_series_regression} as follows:
    
    \begin{itemize}
        \item $R^e_{i,t} = \mathbb{E}_t\left[ \frac{P_{i,d \in t}}{P_{i,d-1}} - (1+R^f_{d \in t}) \right]$, where $d$ is a day in calendar week $t$, $P_{i,d}$ is the closing price of asset $i$ on day $d$, and $R^f_d$ is the daily risk free rate on day $d$,and $\mathbb{E}_t$ computes the arithmetic mean of price returns across days $d$ in week $t$,
        \item $\sigma^e_{i,t} = \sqrt{\mathbb{VAR}_t\left[ \frac{P_{i,d \in t}}{P_{i,d-1}} - (1+R^f_{d \in t}) \right]}$, where $d$ is a day in calendar week $t$, and $\mathbb{VAR}_t$ computes the variance of price returns across days $d$ in week $t$,
        \item $Q_{i,t} = \mathbb{E}_t\left[ P_{i,d \in t} V_{i, d \in t} \right]$, where $V_{i,d}$ is the trading volume, in billions, of asset $i$ on day $d$.
    \end{itemize}
    
    We calculated the variables used in Table \ref{tab:adjacent_sentiment_spillovers} as follows:
    
    \begin{itemize}
        \item $R^e_{i,t} = \frac{P_{i,t}}{P_{i,t-1}} - (1+R^f_t)$, where $P_{i,t}$ is the closing price of asset $i$ on day $t$, and $R^f_t$ is the daily risk free rate on day $t$,
        \item $\widetilde{R^e_{i,t}} = \frac{P_{i,t-1}}{P_{i,t-6}} - (1+R^f_{t-6})^5$, where the 5-period lag is based on a 5-day trading week,
        \item $\sigma_{i,t} = \sqrt{\frac{1}{10}\sum_{k=1}^{11} (R^e_{i,t-k} - \overline{R^e}_{i,t-1})^2}$, where $\overline{R^e}_{i,t}$ denotes the average excess return observed between days $t$ and $t-10$,
        \item $\boldsymbol{W}$ is the normalised submission adjacency matrix, where $w_{i,j}$ is equal to the number of comments made by $i$'s author on an older submission $j$ with the same extracted ticker, divided by the total number of comments made by $i$'s author on older submissions with the same extracted ticker,
        \item $\phi^s$ denotes a dummy variable for a submission with sentiment $s$, where $s$ can be bullish ($s = +1$), bearish ($s = -1$) or neutral ($s = 0$),
        \item $\phi^s_{-1}$ denotes a dummy, as above, for the sentiment of the last post made by the author on the same extracted ticker, where $\phi^{NA}_{-1}$ represents the lack of such a submission.
    \end{itemize}
    
    We took two extra cleaning steps. First, to account for stock splits and mergers, we use CRSP's cumulative factors to adjust prices and volumes for each security $i$. Second, we remove any instances where the price is negative, or the excess return is greater than 10.
