# Supplementary material for: Social contagion and asset prices: Reddit's self-organised bull runs
Source: arXiv:2104.01847 source file (2023-08-08)
Supplement: Supplementary file 9 [file Model_30_Jan_2023.tex]

\section{Social dynamics and asset prices}
\label{sec:model}

Sharing investment strategies appears self-defeating, so what motivates retail investors to do so online, in such an unabashed manner? We study their interactions through an asset demand model, by incorporating information complementarities in investment decisions. These give rise to \textit{social contagion} in asset demand; investors buy the asset because others do as well, irrespective of their personal beliefs. This behaviour, if significant, can create reversals in asset price returns. 

The mechanism is motivated by a recent literature that studies diagnostic expectations \citep{bordalo2021diagnostic}. In doing so, investors trade on the momentum of the stock price, against a supply of shares provided by noise traders.  Our inclusion of a social component subsequently induces persistence in asset demand over time, which leads to reversal in future returns after an increase in price.

\subsection{General setup}
\label{subsec:asset_demand}
We analyse prices in each period $t$ for one asset traded by $N$ investors, indexed by $i$. Each investor derives CARA utility from consuming $c$, $U_i(c_i) = \text{exp}(-\gamma c_i)$, where $\gamma$ is the constant absolute rate of risk aversion. We do not include any discounting in their decision-making, but assume they evaluate the asset according to a forward-looking value $V$ with expectation $\mathbb{E}_i(V)$.

For now, we drop the time subscript to study a static version of the model. Shares $\phi_i$ are purchased at current market price $p$ to optimise the mean-variance objective function \begin{align}
\label{eq:mean_variance_tradeoff}
    \mathcal{L}(\phi_i) &= [\mathbb{E}_i(V) - p]\phi_i - \frac{\gamma}{2}\mathbb{E}_i(V - p)^2\phi_i^2, \\
    \Rightarrow \phi_i^\ast &= \frac{\mathbb{E}_i(V) - p}{\gamma \mathbb{E}_i(V - p)^2},
\end{align}
where an asterisk denotes the value that maximises objective $\mathcal{L}$. In this way, we distinguish between beliefs about value $\mathbb{E}_i(V)$ from investor $i$'s decision to buy amount $\phi_i$. 

\paragraph{Simple price equilibrium} We assume that asset supply originates from noise traders, as in \citet{bordalo2021diagnostic}, to find a price equilibrium. In effect, equilibrium demands $\sum \phi_i^\ast$ sum to exogenous supply $S$. Assuming fixed uncertainty $\sigma^2 = \mathbb{E}_i(V - p)^2$ and averaging expected values $\mathbb{E}(V) = {1}/{N} \sum \mathbb{E}_i(V)$ yields the following expression for the equilibrium price:
\begin{align}
    p = \mathbb{E}(V) - \frac{S}{N} \gamma \sigma^2. \label{eq:simple_equilibrium}
\end{align}
Eq. \ref{eq:simple_equilibrium} accounts for the price level by investor's average expected value of the asset, in addition to their ability to absorb the exogenous level of assets supplied. This ability depends on the depth of the investor pool -- reflected by the number of investors $N$ -- as well as their risk appetite $\gamma \sigma^2$. In this simple market, the price increases with expected value, and decreases with supply.

This expression for prices also ignores heterogeneity and aggregation. Eq. \ref{eq:simple_equilibrium} mimics a single representative investor with some demand size $N$. However, strategic interactions may give rise to feedback loops in investor demands that do not average out. We also do not consider the effect of heterogeneity in investor wealth, or other size metrics, although the model can be extended for that purpose. Investors central in a social network are `indirectly' large by their ability to sway others. [GABAIX]

The first goal of this section is to endogenise investors' expectation formation for value $\mathbb{E}_i(V)$, and determine a trajectory for prices when aggregating these components. A long literature investigates the link between subjective asset price beliefs and prices, and our contribution is to include a term for social learning. The second goal is to investigate this equilibrium price in a dynamic setting where values are updated under some extrapolation.

\subsection{Static model with information complementarities} 
We study the role of information complementarities in investors' beliefs about the value of an asset. Investor $i$'s maximised payoff from Eq. \ref{eq:mean_variance_tradeoff} is
\begin{align}
    \mathcal{L}(\phi_i^\ast) &= \frac{1}{2\gamma} \frac{\mathbb{E}_i^2(V-p)}{\mathbb{E}_i(V-p)^2} \\
    % &= \frac{1}{2\gamma} \left(1 - \frac{\mathbb{E}_i[\mathbb{E}_i(V) - V]^2}{\mathbb{E}_i(V-p)^2}\right),
    &= \frac{1}{2\gamma} \left(1 - \frac{\sigma_i^2(V)}{\mathbb{E}_i(V-p)^2}\right),    
\end{align}
where $\sigma_i^2$ denotes investors' variance for value $\sigma_i^2(V) = \mathbb{E}_i(V^2) - \mathbb{E}_i^2(V)$. At this optimised level, payoffs decrease as uncertainty about value $V$ increases, to the extent that squared returns themselves are low. This expression demonstrates the value of social networking. If investors start with different signals about the asset's value, the ability to aggregate them by listening to others improves the precision of their expectation, and their final expected payoff. In this stage, prices themselves do not feature. Investors benefit from a better estimate of value $V$ at any price $p$.

The extent to which uncertainty on the difference between realised price from the expected value $\mathbb{E}_i(V-p)^2$ is significant remains unclear. Investors expect the price to be a realisation of aggregated expected value and a mean zero, unobserved supply shock $S$. The difficulty in finding a market-clearing price lies in the non-linear aggregation of demand. Price is not linear in the expectations of value, nor in the uncertainty faced by individuals.

To circumvent this problem, we assume a specific form for investors' price uncertainty:
\begin{align}
    E_i(V - p)^2 = \sigma_i^2(V) + \sigma_i^2(s),
\end{align}
where $\sigma_i^2(s)$ corresponds to the variance of supply shock $S \gamma \sigma^2 /N$ in Eq. \ref{eq:simple_equilibrium}. This form for uncertainty corresponds to an investor who based their price expectations on a form of the simple equilibrium in Eq. \ref{eq:simple_equilibrium}, but uses their expected value as the aggregate, and does not adjust their 


An investor's expectation includes some signal $b_i$, with information both public and private to $i$, and asset demand by other investors $\phi_{-i}$:
\begin{align}
    \mathbb{E}_i(V) = g(b_i) + f(\phi_{-i}).
    \label{eq:quadratic_loss}
\end{align}
We assume that functions $g(\cdot),f(\cdot)$ are monotonic and continuous, but are specifically interested in the form of $f(\cdot)$. Eq. \ref{eq:quadratic_loss} is a well-known formulation for strategic interactions between agents acting under quadratic loss \citep{zenou2016key}. Definition \ref{definition:complementariy} establishes the notion of complementary investment in this context.

\input{Cells/1_Definition}

The complementarity in asset demand between investors comes from the aggregation of idiosyncratic information on the value of the asset. Investor $i$ is motivated to better inform their decision by gleaning information from their peers' actions. Thus, if they believe the value is low due to their personal signal $b_i$, higher purchases by their friends would lead them to revise their decision to buy a low amount of the asset. The investor in question may have simply drawn a bad signal. Here, we simplify the analysis by assuming that each investor's information aggregation method is an arithmetic mean of others' investment demand. The asset's expected value increase linearly in this `social' component. Information acquisition under complementary decisions is studied in detail by \citet{hellwig2009knowing}.

\paragraph{Strategic complementarities and peer effects.}
What compels retail investors to share strategies via WSB? We suggest one answer by appealing to \cites{hellwig2009knowing} main result, which we rewrite in Proposition \ref{proposition:strategic_interactions}. In addition to the quadratic loss assumed in Eq. \ref{eq:mean_variance_tradeoff}, we remind the reader of the additional assumptions in their framework, adapted to the present context.
\input{Cells/1_Assumption}
\input{Cells/2_Assumption}
\input{Cells/1_Proposition}

Proposition \ref{proposition:strategic_interactions} predicts that interactions between investors whose decisions include a social component (a group we call `hype investors') provide them with additional expected utility. This, in turn, increases their propensity to invest according to their updated sentiment, under costly information acquisition. We empirically validate whether Proposition \ref{proposition:strategic_interactions} holds in the context of WSB and, thereby, study the social aspects of investing. 

\subsection{Price dynamics with peer effects} 

To study the joint dynamics of an asset's price and demand by social investors, we treat demand $\phi$ and price $p$ as state variables for a dynamic system, indexed by time $t$. In doing so, we assume that demands $\phi_{i,t}$ are updated using signals $b_{i,t}$ and past demand $\phi_{t-1}$. Aggregate asset demand and price are
\begin{align}
    \phi_t &= \frac{\mathbb{E}_t[g(b_{i,t})] + \alpha \phi_{t-1} - p_t}{\gamma \sigma^2}, \label{eq:demand_system} \\
    p_t &= \mathbb{E}_t[g(b_{i,t})] + \alpha \phi_{t-1} - \frac{S_t}{N}\gamma \sigma^2, \label{eq:price_system}
\end{align}
which demonstrate the importance of signals $b_{i,t}$ in determining the trajectory of demand. Studies in behavioural finance suggest several components that ultimately deviate from rational expectations. In this instance, demand depends on it's lag. We believe this accurately reflects the nature of discussions on WSB specifically, which is characterised by `leaders' who garner followers to adopt their positions. 

% \paragraph{Rational Expectations.} For the simplest scenario, we make the first assumption that investors value the asset according to its expected future price, so that $\mathbb{E}[g(b_{i,t})] = \mathbb{E}_t(p_{t+1})$. This leaves us with an easy system to analyse:
% \begin{align}
%     \phi_t &= \frac{\mathbb{E}_t(r_{t+1}) + \alpha \phi_{t-1}}{\gamma \sigma^2}, \\
%     \mathbb{E}_t(r_{t+1}) &= - \alpha \phi_{t-1} + \gamma \sigma^2 \phi_t ,
% \end{align}
% where return $r_t \equiv p_t-p_{t-1}$. The expression for returns in terms of asset demand can be simplified to 
% \begin{align}
%     \mathbb{E}_t(r_{t+1}) = \gamma\sigma^2 \Delta \phi_t + (\gamma\sigma^2 - \alpha) \phi_{t-1},
% \end{align}
% where $\Delta x_t \equiv x_t - x_{t-1}$. 

\paragraph{Mechanical Extrapolation.} We assume that investors partially trade on the momentum of the asset's price, which \citet{bordalo2021diagnostic} term `mechanical extrapolation'. The functional form of $\mathbb{E}[g(b_i)]$ is specified in Assumption \ref{assumption:mech_extrapolation}.

\input{Cells/1.1_Assumption}

Mechanical extrapolation is our preferred way to introduce a relationship between prices and demand \citep{barberis2018extrapolation}. A model with mechanical extrapolation has several shortcomings, one of which is the inability to relate expectation updates to psychological underpinnings. However, our assumption is justified by our empirical work in Section \ref{sec:consensus_results} which demonstrates that individuals update their outlook based on recent asset returns. 

\paragraph{System for price and demand.} Substituting Eq. \ref{eq:mech_extrapolation} into Eqs. \ref{eq:demand_system}-\ref{eq:price_system} yields demands and prices
\begin{align}
    \phi_t &= \frac{\alpha \phi_{t-1} + \beta r_t}{\gamma \sigma^2}, \\
    r_t &= -\frac{\alpha}{\beta} \phi_{t-1} + \frac{S_t\gamma \sigma^2}{\beta N}.
\end{align}
In this scenario, asset demand and returns are determined simultaneously. The first mechanism is through market clearing, where demand has to adjust to supply. The second is the adjustment of the expected value for the asset to the realised return through $\beta$ and the social signal through $\alpha$. As a result, returns are accounted for by current and past asset demand:
\begin{align}
\label{eq:return_against_demand}
    r_t = \frac{\gamma\sigma^2 }{\beta} \phi_t - \frac{\alpha}{\beta} \phi_{t-1}.
\end{align}
% \begin{align}
%     r_t = \frac{\gamma\sigma^2 }{\beta}\Delta \phi_t + \frac{\gamma\sigma^2 -\alpha}{\beta} \phi_{t-1}.
% \end{align}
This equation for asset demand in equilibrium offers three valuable insights. First, it requires a non-zero degree of extrapolation $\beta > 0$, otherwise demand does not adjust to price. Investors are never compelled to change their purchases since they believe the current price precisely reflects value. Second, higher demand increases current returns, but leads to a subsequent reversal in the following period. This is because the equilibrium price needs to satisfy the value expected both from extrapolation, in addition to the value estimated from the social components. Under exogenous supply, a strong positive signal from peers means that the extrapolated return is \textit{less} important in justifying a higher price. In equilibrium, this results in a negative relationship between returns and the lag in asset demand.

The reversal in returns is an important feature that emerges from social contagion in investors' price expectations. If large enough, these can produce bubbles in asset prices: initial momentum from positive news creates a price run-up, before an absence of news creates a drought of new asset demand. The subsequent price crash carries on its own momentum. We can treat demand as a latent variable to see these oscillations manifest in return data. Substituting lagged demand into the equation for returns, and iterating infinitely yields
\begin{align}
\label{eq:return_time_series}
    r_t = -\sum_{T = 1}^\infty \left(\frac{\alpha}{\gamma \sigma^2}\right)^T r_{t-T} + \frac{S_t\gamma \sigma^2}{\beta N}
\end{align}
as long as $\alpha / \gamma \sigma^2 < 1$, so that the contribution of demand fluctuations to returns converges to zero over time. This is an autoregressive model with infinite lags, where the coefficients decrease exponentially with lag size $T$. Without any knowledge of asset demand, the second term encapsulates an unobservable error term which the model links to exogenous changes in the asset's supply. Eq. \ref{eq:return_time_series} demonstrates that an exogenous increase in returns at time $t$ is followed by an smaller decrease in $t+1$. This oscillation persists indefinitely, and would converge to zero rapidly if the social signal $\alpha / \gamma \sigma^2$ is sufficiently small.

\subsection{Full model with fundamental traders.} 
\label{sec:model_bubbles}

The previous section proposes a simple model for how an economy with a single investor type, who extrapolate past price movements and leverage the sentiment of peers to determine asset demand. This model informs the potential relationship we can expect between returns and observed investor sentiment online. However, how would asset prices dynamically evolve in an economy with both `fundamental' traders and those who trade based on sentiment (formed from peers and extrapolation)? We further develop a model from \cite{barberis2018extrapolation} to understand how market dynamics might develop.

\paragraph{Investor price expectations} We begin with the same investment setting as \cite{barberis2018extrapolation}. We consider an economy with T + 1 dates. There are two assets: one risk-free and one
risky. The risk-free asset earns a constant return which we normalize to zero. The risky asset has a fixed supply of Q shares, and each share is a claim to a dividend $D_T$ paid at
the final date, T. The value of D is determined by $D_0$, a final dividend paid at time T whose value is known, and $N(0, \sigma^2_{D})$, which is i.i.d. noise realize at each time period. The price of the risky asset, $P_t$, is determined endogenously. There are two types of traders in the economy: fundamental traders and `hype' investors whose investment decisions are marked by $F$ and $H$. The time $t$ per capita demand of fundamental traders for shares of the risky asset is:
\begin{align}
    \frac{D_t - \gamma\sigma^2_{D} (T-t-1)Q - P_t}{\gamma\sigma^2_{D}},
\end{align}
where $D_t$ is the sum of $D_0$ and realized shocks to the dividend up to time $t$ and $\gamma$ is the trader's risk aversion. This expression is consistent with an investor who maximises a CARA utility defined ove r the next period's wealth.  

Hype investor demand, on the other hand, place some weight on the fundamental signal, but also place some weight on past price changes and the sentiments of others (in an effort to reach strategic information complementarities, as described in \cite{hellwig2009knowing}:

\begin{align}
    w_H \frac{D_t - \gamma\sigma^2_{D} (T-t-1)Q - P_t}{\gamma\sigma^2_{D}} + (1 - w_H)\frac{X_t}{\gamma\sigma^2_{D}},
\end{align}
where $X_t$ is the `hype' signal at time $t$. We propose two versions of the hype signal: i) where the hype investor updates his demand based on past stock returns and the observed sentiments of other investors, $X_t^d$, and ii) where the the hype investor updates his belief about the future price change of the stock, rather than demand, $X_t^b$. Both models are of interest since the former is more directly comparable to the literature, while the latter is closer to the parameters we can estimate from the data. 

$X_t^d$ is updated as follows:
\begin{align}
    \label{eq:X_update_demand}
    X_{t}^d = \theta_d X_{t-1}^d + (1-\theta_d)S_t,
\end{align}
where $S_t$ is the investor sentiment composed of the observed sentiment of peers in the previous time step, $S_{t-1}$, and the observed price change, $P_{t-1} - P_{t-2}$,
\begin{align*}
    S_t = w_E(P_{t-1} - P_{t-2}) + w_S(S_{t-1}).
\end{align*}
This modeling choice implies that individual demand is driven not only by changes in price, but also in how fellow hype investors react. The model also gives additional flexibility to explore how assets might react to a purely socially-driven shock, rather than only a new-driven one.

 $X_t^b$ is updated as follows:
\begin{align}
    \label{eq:X_update_belief}
    X_{t-1}^b = \theta_b B_{t-1} + (1-\theta_b)S_t,
\end{align}
where $S_t$ is defined as before, but the investor updates their entire belief about the change in asset price, rather than only the `hype' part of his belief,
\begin{align*}
    B_t = w_H \frac{D_t - \gamma\sigma^2_{D} (T-t-1)Q - P_t}{\gamma\sigma^2_{D}} + (1 - w_H)\frac{X_t^b}{\gamma\sigma^2_{D}}.
\end{align*}
In the formulation with beliefs, we are able to measure the expressed sentiments of investors online over time and estimate $\theta_b$ based on the information they are exposed to and how their sentiment is updated. This is not possible when we do not explicitly estimate the investor belief, as in the formulation in \ref{eq:X_update_demand}.

\paragraph{Determining a market-clearing price.} As in \cite{barberis2018extrapolation}, we propose a short sale constraint to establish the market-clearing price, where the quantity demanded by both types of traders is bounded at zero:
\begin{align}
    \label{eq:short_sale}
    N_t^F &= max \left[   \frac{D_t - \gamma\sigma^2_{D} (T-t-1)Q - P_t}{\gamma\sigma^2_{D}}, 0 \right], \\
    N_t^H &= max \left[  w_H \frac{D_t - \gamma\sigma^2_{D} (T-t-1)Q - P_t}{\gamma\sigma^2_{D}} + (1 - w_H) \left(\frac{X_t}{\gamma\sigma^2_{D}} \right) , 0 \right].    
\end{align}
We use this formulation to calculate the price at which the short-sale constraint begins to bind for each type of trader -- at this price the trader would be indifferent between staying in or leaving the market:
\begin{align}
    \label{eq:market_clearing}
    P_t^F &= D_t - \gamma\sigma^2_{D} (T-t-1)Q - P_t, \\
    P_t^H &= D_t - \gamma\sigma^2_{D} (T-t-1)Q - P_t + \frac{(1 - w_H)}{w_H} \left(\frac{X_t}{\gamma\sigma^2_{D}} \right). 
\end{align}
Finally, we calculate the total demand at both price points, $P_t^F$ and $P_t^H$. If the quantity demanded at both price points is below Q, the total number of shares available, we determine the price as if both types of traders were in the market -- as shown in Eq. \ref{eq:bubble_price1}. Otherwise, we determine the price as if only hype traders were in the market, as in Eq. \ref{eq:bubble_price2}:
\begin{align}
    \label{eq:bubble_price1}
    P_t &=  D_t + \frac{\mu_H(1-w_H)}{\mu_F+\mu_H w_H} X_t - \gamma \sigma_D^2 Q \frac{(T-t-1) (\mu_H w_H + \mu_F) + 1}{\mu_H w_H + \mu_F},\\ 
    \label{eq:bubble_price2}
    P_t &=  D_t + \frac{\mu_H(1-w_H)}{\mu_H w_H} X_t - \gamma \sigma_D^2 Q \frac{(T-t-1) (\mu_H w_H) + 1}{\mu_H w_H}.
\end{align}

\paragraph{Bubbles and peers}

We compare the price dynamics across different models for bubbles. As a first baseline model, we consider the market price if all traders were fundamental traders. The market clearing price would be: 
\begin{align*}
    D_t - \gamma \sigma_D^2(T-t-1)Q.
\end{align*}
As a second baseline, we consider the model from \cite{barberis2018extrapolation}, which is similar to our model in for $X_t^d$ in Eq. \ref{eq:X_update_demand}. We look to compare our two baseline models to our model for hype investor demand, where $X_t^d$ is updated as in Eq. \ref{eq:X_update_demand}, and our model for hype investor beliefs, where $X_t^b$ is updated as in Eq. \ref{eq:X_update_belief}.


    \begin{figure}[!ht]
        \centering
        \includegraphics[width = 0.95\textwidth]{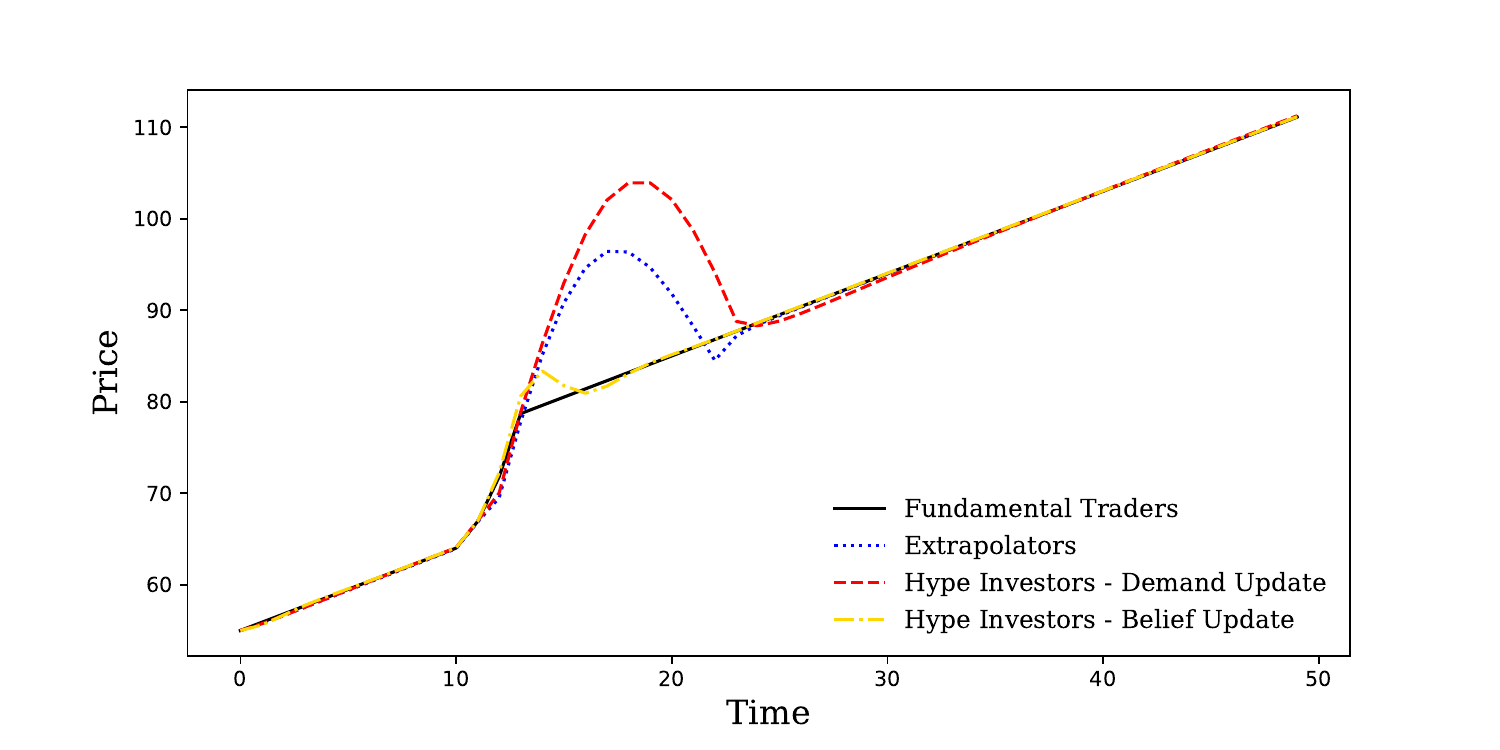}
        \caption{\footnotesize{\textbf{Bubbles with Hype Investors:} We present the price evolution for an asset in several settings: i) with only 
 fundamental traders are present, ii) with fundamental traders and extrapolators \citep{barberis2018extrapolation}, iii) with fundamental traders and hype traders who update their demand, and iv) with fundamental traders and hype investors who update their beliefs. We observe the asset over 50 time periods (T=50), which has $D_0 = 100$ and experiences 10 shocks of zero, followed
by shocks of 2, 4, 6, followed by 37 shocks of zero to its dividend. We assume 30\% of traders are fundamental traders, $\mu_F$, and 70\% are non fundamental, $\mu_H$ (except for the \textit{Fundamental Traders} model, where all traders are assumed to be fundamental). Other parameters in the model are: $\sigma_D = 3$, $\gamma = 1$. For the models of \textit{Extrapolators} and \textit{Hype Investor - Demand Update}, we set $\theta$ and $\theta_d$ to 0.9, and $w_i$ and $w_H$ to 0.1. For both hype investor models, we set $w_E$ and $w_S$ to 0.9 and 0.2, respectively, as shown by the data. For our model of \textit{Hype Investor - Belief Update} we set $\theta_b$ to 0.15, and $w_E$ to 0.6 as motivated by our data. }}
        \label{fig:bubbles1}
    \end{figure}

For our first experiments, presented in Figure \ref{fig:bubbles1}, we consider a setting similar to \cite{barberis2018extrapolation}. We observe 50-period
sequence of cash-flow shocks impacting the dividend at each time $t$ (T=50), where $D_0$ is known to be 100. The first ten shocks are all equal to zero, followed by three positive shocks (2, 4, 6), followed by 37 more shocks of zero. We motivate our choice of parameters for the models of hype investors by our observations from our empirical work in the following section. Specifically, we observe that investors place significant weight on the extrapolation and therefore set $w_E = 0.9$; they also update their perspectives based on peers and set $w_S = 0.2$. We are not able to observe how hype investors update their demand -- we therefore set $\theta_d = 0.9$ consistently with \cite{barberis2018extrapolation}, however, we are able to observe changes to their belief. We, therefore, estimate $\theta_b = 0.15$ -- showing that investors place a much greater weight on recent information than on their past beliefs. Finally, we observe that peer sentiments and recent extrapolation explain a fraction of how investors update their beliefs -- we, therefore, conclude that hype investors likely place a greater weight on fundamental signals than assumed in \cite{barberis2018extrapolation} and set $w_H = 0.6$ for our model with belief updates. 

There are several noteworthy observations from Figure \ref{fig:bubbles1}. A model with peers creates larger and more prolonged bubbles than that without - observable by comparing the model with \textit{Extrapolators} and \textit{Hype Investors - Demand Update}. This is unsurprising as price increases are driven not only by extrapolation, but also by peer reinforcement who reinforce the validity of the price increase. We also observe that our model with belief updates produces a much shorter price deviation. This is largely caused by the greater emphasis that traders in this model place on the fundamental value of the asset. We believe that this, however, seems like a plausible model -- the change in the dividend corresponds to a single shock over two standard deviations. Even though it is likely that the market might over-react in such a scenario, we would not necessarily expect a prolonged bubble from a single shock of this size. 

    \begin{figure}[!ht]
        \centering
        \includegraphics[width = 0.95\textwidth]{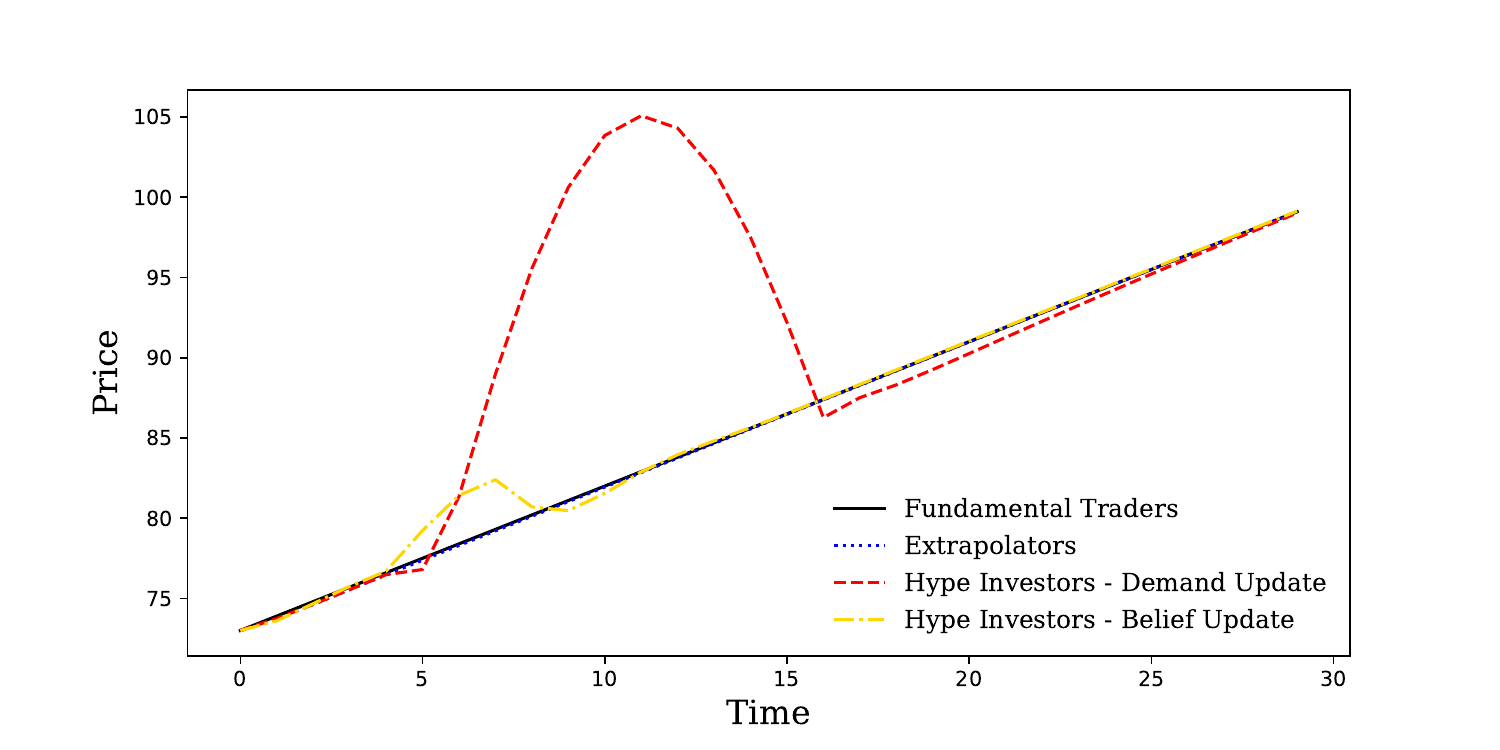}
        \caption{\footnotesize{\textbf{Bubbles with Hype Investors:} We present the price evolution for an asset in several settings: i) with only 
 fundamental traders are present, ii) with fundamental traders and extrapolators \citep{barberis2018extrapolation}, iii) with fundamental traders and hype traders who update their demand, and iv) with fundamental traders and hype investors who update their beliefs. We observe the asset over 30 time periods (T=50), which has $D_0 = 100$ and experiences no dividend shocks, however, experiences positive peer sentiment shocks of 20 in periods 5,6,7. We assume 30\% of traders are fundamental traders, $\mu_F$, and 70\% are non fundamental, $\mu_H$ (except for the \textit{Fundamental Traders} model, where all traders are assumed to be fundamental). Other parameters in the model are: $\sigma_D = 3$, $\gamma = 1$. For the models of \textit{Extrapolators} and \textit{Hype Investor - Demand Update}, we set $\theta$ and $\theta_d$ to 0.9, and $w_i$ and $w_H$ to 0.1. For both hype investor models, we set $w_E$ and $w_S$ to 0.9 and 0.2, respectively, as shown by the data. For our model of \textit{Hype Investor - Belief Update} we set $\theta_b$ to 0.15, and $w_E$ to 0.6 as motivated by our data. }}
        \label{fig:bubbles2}
    \end{figure}

    For our second set of experiments, we would like to show how `animal spirits' or a random positive shock to peer sentiments can also drive bubbles. In Figure \ref{fig:bubbles2}, we show that several positive shocks to peer sentiment can, indeed, drive prices to deviate from fundamentals in our model. The individuals react more quickly, in our model with belief updates and the price returns to its fundamental value more rapidly, as hype traders place a greater emphasis on fundamental value. 

\subsection{Initial evidence}
