# Supplementary material for: Social contagion and asset prices: Reddit's self-organised bull runs
Source: arXiv:2104.01847 source file (2023-08-08)
Supplement: Supplementary file 10 [file VAB_model.tex]

\newpage

\subsection{Contagion Model}
\label{app:vab_model}

\paragraph{Contagion}
    We turn to an adapted Kermack-McKendrick SIR epidemic model to quantify the evolution of asset demand via social contagion, advocated in \citet{shiller2017narrative}. This choice is justified through our results in Section \ref{subsec:contagion} and empirically validated in Appendix \ref{app:vab_model}. We propose the following relationships between susceptible, $V$, active/infected, $A$, and recovered, $B$, investors in a specific asset:
    \begin{align}
    \label{eq:sir}
        \frac{dV}{dt} &= -cAV, \\
        \frac{dA}{dt} &= cAV -rA, \nonumber \\
        \frac{dB}{dt} &= rA, \nonumber
    \end{align}
    where $c$ is the contagion rate, and $r$ is the recovery rate. The total population of potential hype investors, $N=V+A+B$, is assumed constant. We take this model literally to understand contagion in asset interest on WSB. `Active' users forgo passive investment, adopt a specific position in an asset, and convince others to do the same. `Recovered' users lose interest and cease to believe in the hype, and thus close their asset-specific position. `Susceptible' users have not yet taken any investment action but could potentially become interested in the asset, as they seek investment advice from their peers. We use $A$ as an estimate for the number of hype investors in an asset at a certain point in time. 

\paragraph{Empirical evidence for the contagion model}
    
 %       \begin{figure}[ht]
 %                   \centering
 %                   \includegraphics[width=\textwidth]{Figures/VAB/all_ticker_activity.pdf}
 %                   \caption{\textbf{Ticker Activity versus Overall WSB Activity}; the number of unique monthly active users (users who comment or post) on the left y-axis plotted plotted against the unique number of posters about a specific ticker (on the right y-axis). Both are plotted as 3-month rolling means.}
 %                   \label{fig:contagion_activity2}
 %       \end{figure}

        \begin{figure}[ht]
            \begin{subfigure}[t]{.5\textwidth}
                \centering
                \includegraphics[width=\textwidth]{Figures/VAB/JNUG.pdf}
                \subcaption{JNUG}
                \label{fig:vab_jnug}
            \end{subfigure}
            \begin{subfigure}[t]{.5\textwidth}
                \centering
                \includegraphics[width=\textwidth]{Figures/VAB/MU.pdf}
                \subcaption{MU}
                \label{fig:vab_mu}
            \end{subfigure}  
            \bigskip
            \begin{subfigure}[t]{.495\textwidth}
                \centering
                \includegraphics[width=\textwidth]{Figures/VAB/SNAP.pdf}
                \subcaption{SNAP}
                \label{fig:vab_snap}
            \end{subfigure}  
            \hfill \hfill 
            \begin{subfigure}[t]{.495\textwidth}
                \centering
                \includegraphics[width=\textwidth]{Figures/VAB/TSLA.pdf}
                \subcaption{TSLA}
                \label{fig:vab_tsla}
            \end{subfigure}
            \caption{\textbf{Contagion Model Forecasts for Active Investors in Assets on the WSB Forum}; the contagion model is initialized with the parameters at the start of an `outbreak' of activity on WSB in a specific ticker and used to approximate the growing interest and, subsequent, loss of interest.}
            \label{fig:VAB_model_applied}
        \end{figure}
        We provide evidence that discussions about assets are self-perpetuating on WSB: social contagion appears to play a role in the assets that investors discuss and consider for their portfolios. Here, we attempt to reconcile the size of discussions on WSB over time with our contagion model of choice: the epidemiological SIR model.
        
    Figure \ref{fig:contagion_activity} shows that some of the most commonly mentioned tickers appear to exhibit a hump-shaped pattern of number of interested users over time. We use data from WSB to estimate our contagion parameters, $c$ and $r$, at different points in time and show that our simple contagion model captures the hump-shaped ticker interest. One challenge is that our epidemic model is well-suited to model a single `outbreak' in ticker interest, as it assumes a static population. We, therefore, look at how well our model fits data with non-overlapping periods of discussion intensity.
        
    Figure \ref{fig:VAB_model_applied} shows the \textit{predicted} discussion sizes of specific tickers from the contagion model (as a percent of active users on the forum at the time) versus the \textit{actual} sizes of ticker discussions on the WSB forum. Despite its clear shortcomings, this simple model that is tuned on noisy global parameters still captures the overall shape of social contagion in ticker interest. It exhibits some desirable properties, such as the fact that contagion spreads more slowly in communities that are sparse and faster as the community grows: consider Figure \ref{fig:vab_jnug} where JNUG interest gradually permeated the forum over the course of a year, whereas TSLA interest in 2020, displayed in Figure \ref{fig:vab_tsla}, spread to a much greater population over the course of three months.

\paragraph{Estimating $c$ and $r$ Parameters Globally}
        Certain contagion variables are more straightforward to estimate from WSB data than others. For the moment, we assume the total population at a given time, $N_t$, to be the number of active users on the forum: those who comment or post at time $t$. The number of users initially interested in asset $i$, $A_{i,0}$, is estimated as the number of people who post about $i$ in some starting period 0. The average dollar amount each user has at their disposal, $M$, can approximated from available surveys\footnote{\url{https://andriymulyar.com/blog/how-a-subreddit-made-millions-from-covid19}}. Model sensitivity is tested against all of these parameters. 
        
        Contagion parameters, $c$ and $r$, require more care in isolating the effect of social interaction from other variables that may impact asset interest. 
        
        The contagion rate is comprised of two parameters: 
        \begin{align}
            c = \tau \gamma,
        \end{align}
        where $\tau$ is transmissibility, the probability of transmission of asset interest given contact between a susceptible and active investor), and $\gamma$ the average rate of contact between susceptible and active investors on the forum. The first, $\tau$ is easily estimated from the results in Section \ref{subsec:contagion} (further detailed in \ref{app:matching}) showing a spread of ticker-specific interest at a rate of 1.1\% among tail tickers. In order to estimate $\gamma$, we counted the total number of unique users who commented on a submission, on average (this is an approximation for the number of `susceptible' individuals that an infected person comes in contact with), multiplied by the number of posts that a user makes, on average, about a given ticker, and divided by the number of users active on the forum, measured as unique users who post a submission or comment, while the submissions about the ticker are discussed on the forum. We consider interactions to be uniform over the duration of the `infectious period' so divide this number by the duration. The average contact rate is estimated at $\gamma = 1.2\times 10^{-4}\%$. This may seem particularly small, however, intuitively this is not surprising as $\gamma$ captures how many people will pay attention to a single submission versus all the other content in a thriving online community. The contact rate also differs greatly from one month to the next as people join and leave the forum, so this rate is more precisely tracked for each ticker that we estimate contagion for. This returns a combined contagion rate of $c = 9.8 \times 10^{-7}$.
        
        Estimating $r$ presents a challenge: users do not advertise a loss of interest in an asset on WSB. In order to estimate the recovery rate, we turn to its classic definition as `the inverse of the infectious period,' as described in \cite{ridenhour2018unraveling}. We consider the `infectious period' the time difference between when an author make his first post about a ticker and the time when his last post ceases to receive comments (ceases to be actively discussed on the forum). During this period, an individual spreads their perspective about an asset on the forum. We estimate the recovery rate at approximately $r = 1/19.6 = 5.1 \times 10^{-2}$. 
        
\paragraph{Initializing $c$, $r$, $N_0$ and $A_0$ for Social Contagion in a Specific Ticker}
        In order to estimate the contagion patterns presented in Figure \ref{fig:VAB_model_applied}, we tune the contagion parameters to be more precise for the ticker and time period in question. We initialize $N_0$ as the total number of unique authors who are active on the forum from the start to five months after the beginning of the contagion: we select this period in order to estimate the size of the population who would be affected by the excitement about a ticker, but we make the period sufficiently short so as to avoid capturing inflated population numbers driven by user churn (when a group of users becomes uninterested in a given subreddit and is replaced by a new group of users). One important shortcoming which results from this modeling choice is the fact that the model consistently over-estimates the number of infected individuals: our initial $N_0$ contains all posters and commenters on the forum; however, Section \ref{sec:data_method} establishes that there is an order of magnitude more comments than posts on the forum. Ultimately, we are interested in tracking posters in a given asset; this difference in populations results in consistent over-estimation. We initiate $A_0$, the initial population that begins to discuss a ticker on the forum driving further interest, as the average number of of unique authors posting about the ticker in the three months preceding the uptick. We also adjust $\gamma$ to be calculated at the time the uptick begins.

%\paragraph{Units and Further Discussion on Initialization of Parameters}

%We check our contagion units with the standard epidemeology literature and intuition. The change equations in Eq. \ref{eq:sir} should result in a unit of: $\frac{persons}{day}$. We consider our input into the $c$ constant; we know that $A,V$ have a units of $persons \times persons$, therefore our $c$ constant must have units of $\frac{1}{person-day}$. Our $c$ constant is composed of $\tau$ and $\gamma$. $\gamma$ helps us quantify how many contacts occur between $passive$ and $active$ individuals each day; $\tau$ tells us what proportion of the $passive$ investors become $active$ as a result. $\tau$ is a unitless constant as it is in persons who become $active$ divided by persons contacted in total, or $\frac{persons}{persons}$. The $\gamma \times AV$ should give us the total contacts between $passive$ and $active$ per day in units $\frac{person}{day}$. $\gamma$ should give us, for every $active$ individual, on a given day they are active, what is the probability that a $passive$ person comes in contact with them (in units of 1 divided by person $\times$ day)? Subsequently, $\gamma \times A$ would give us the number of $active$ investors that a single $passive$ investor comes into contact with each day. Finally, $\gamma \times AV$ would give us the total contacts between the two. We, therefore approximate $\gamma$ with this in mind. The $\gamma$ parameter is sometimes referred to as the fraction of $active$ individuals that a passive individual comes in contact with. However, on the WSB forum, the fraction of $active$ individuals is relatively small compared to the overall population. We therefore estimate the fraction of active individuals as the probability to come in contact with a single active individual (essentially discounting the probability that a $passive$ individual will encounter multiple $active$ individuals in a given day). This decision is justified both given how few $active$ individuals there are as compared to the overall size of the forum and given that in Figure \ref{fig:contagion_plot} we show that 71\% of people interact with one post before posting themselves. (or becoming $active$). We consider, over the duration of an $active$ individual posting on the forum, what fraction of the $passive$ population come in contact with this individual. We divide this by the total number of days that the activity lasts (to add a time dimension).

%\paragraph{Sensitivity of the Maximum of Active Investors to $c$, $r$}

%\begin{figure}[ht]
%    \centering
%    \includegraphics[width=\textwidth]{Figures/VAB/beta_gamma_sensitivity.pdf}
%    \caption{\textbf{Sensitivity of $\text{max}(A)$ to $c$ and $r$ Parameters}; this plot shows the dependence of our $\text{max}(A)$ on various initialization parameters. This plot highlights that the current estimate lies at a point with a large gradient where $\text{max}(A)$ is not 0 but also not the entire population. This is consistent with empirical observations where not all investors become interested in a given asset - even for assets which are most popular on the forum. }
%    \label{fig:beta_gamma_sens}
%\end{figure}

%In our model, we are most interest in the number of \textit{active} investors, $A$, at a given point in time. This quantity approximates how many retail investors that are susceptible to social contagion are actively interested and investing in a given asset at a point in time. Specifically, we are interested in the $\text{max}(A)$ over the course of an entire ``social epidemic" as this would be tied to the maximum market impact that the social contagion would have. We, therefore consider how $\text{max}(A)$ varies with our initial $c$ and $r$ parameters. We initialize our model with the parameters in our second Tesla discussion, plotted in Figure \ref{fig:vab_tsla} and observe how $\text{max}(A)$ changes in the surrounding regions for $c$ and $r$, plotted in Figure \ref{fig:beta_gamma_sens}. We observe that as $r$ increases (which is the inverse of the duration for which an investor remains interested in a given asset) the $\text{max}(A)$ decreases: as people loose interest quickly, they have less time to spread their interest to others and, therefore, the excitement in the given asset dies out with very few active investors at a given point in time. We also observe that as $c$ increases, which is our contagion rate, the number of active investors at a point in time increases. A final important point is that a fairly rough approximation for the $c$ and $r$ parameters from our data place the estimate in a ``critical region" of the graph: a region with a high gradient - a region where not all investors on the forum become active in the specified asset. This is intuitive as we do not observe that all investors discuss a single asset; rather a variety of assets are always discussed with different investors becoming part of different ticker discussions. 

%\paragraph{Sensitivity of Contagion Dynamics to $A_0$}

%\begin{figure}[ht]
%    \centering
%    \includegraphics[width=\textwidth]{Figures/VAB/A0_sensitivity.pdf}
%    \caption{\textbf{Sensitivity of Investor Dynamics to $A_0$}; this plot shows that the dynamics are relatively insensitive to how we initialize $A_0$. }
%    \label{fig:A0_sens}
%\end{figure}

%We also consider how dynamics develop for different choices of $A_0$, the number of initial investors who become interested and spread interest in an asset, and plot the evolution for two different values of $A_0$ in Figure \ref{fig:A0_sens} while keeping all other parameters constant. The model appears relatively insensitive to this parameter. A change of $A_0$ from 80 to 10,000 drives only a modest change in the evolution of aggregate investor interest. Interest spreads faster in the latter, however, $\text{max}(A)$ appears relatively consistent demonstrating that other parameters contribute more significantly to $\text{max}(A)$ and the overall dynamics. The graph with $A_0$ highlights a potential flaw with the model; when the right epidemic conditions are met, even a small number of $active$ individuals can trigger a large surge of interest. However, our parameters are extracted from a ticker and time when social contagion in $TSLA$ does occur. The spread of interest is not a given for all initialization parameters and, in fact, is relatively rare. 

%\paragraph{Sensitivity of Contagion Dynamics to $N_0$}

%\begin{figure}[ht]
%    \centering
%    \includegraphics[width=\textwidth]{Figures/VAB/N0_sensitivity.pdf}
%    \caption{\textbf{Sensitivity of Investor Dynamics to $N_0$}; this plot shows that the dynamics are highly sensitive to how we initialize $N_0$. A larger $N_0$ results in a disproportionate increase in $\text{max}(A_0)$ and a fast development of the dynamics. }
%    \label{fig:N0_sens}
%\end{figure}

%In WSB, we have a changing population (which we alter in our initialization for the model presented in Figure \ref{fig:VAB_model_applied}). We observe how dynamics develop for a different $N_0$, while keeping all other parameters constants, in Figure  \ref{fig:N0_sens}. Our model appears highly sensitive to this parameter. Even though in the end, the interest spreads to a total number of investors that is proportional to the increase in $N_0$ (this is observed in the final number of \textit{bored} individuals), the interest spreads much quickly for a large $N_0$. This is particularly important as this is tied to a larger $\text{max}(A)$ and a larger potential market impact generated by the discussion.

\clearpage
